# Supplementary material for: Chiral Phonons with Giant Magnetic Moments in a Topological Crystalline Insulator
Source: arXiv:2208.12235 ancillary file (2023-01-16)
Supplement: Supplementary file 1 [file PbSnTe-SM.pdf]

# Supplementary material for: “Chiral Phonons with Giant Magnetic Moments in a Topological Crystalline Insulator”

Felix G. G. Hernandez,<sup>1</sup> Andrey Baydin,<sup>2,3</sup> Swati Chaudhary,<sup>4,5,6</sup> Fuyang Tay,<sup>2,7</sup> Ikufumi Katayama,<sup>8</sup> Jun Takeda,<sup>8</sup> Hiroyuki Nojiri,<sup>9</sup> Anderson K. Okazaki,<sup>10</sup> Paulo H. O. Rappl,<sup>10</sup> Eduardo Abramof,<sup>10</sup> Martin Rodriguez-Vega,<sup>4,5</sup> Gregory A. Fiete,<sup>5,6</sup> and Junichiro Kono<sup>2,3,11,12</sup>

<sup>1</sup>*Instituto de Física, Universidade de São Paulo, São Paulo, SP 05508-090, Brazil\**

<sup>2</sup>*Department of Electrical and Computer Engineering, Rice University, Houston, Texas 77005, USA*

<sup>3</sup>*Smalley-Curl Institute, Rice University, Houston, Texas, 77005, USA*

<sup>4</sup>*Department of Physics, The University of Texas at Austin, Austin, Texas 78712, USA*

<sup>5</sup>*Department of Physics, Northeastern University, Boston, Massachusetts 02115, USA*

<sup>6</sup>*Department of Physics, Massachusetts Institute of Technology, Cambridge, Massachusetts 02139, USA*

<sup>7</sup>*Applied Physics Graduate Program, Smalley-Curl Institute, Rice University, Houston, Texas, 77005, USA*

<sup>8</sup>*Department of Physics, Graduate School of Engineering Science, Yokohama National University, Yokohama 240-8501, Japan*

<sup>9</sup>*Institute for Materials Research, Tohoku University, Sendai 980-8577, Japan*

<sup>10</sup>*Instituto Nacional de Pesquisas Espaciais, São José dos Campos, SP 12201-970, Brazil*

<sup>11</sup>*Department of Physics and Astronomy, Rice University, Houston, Texas 77005, USA*

<sup>12</sup>*Department of Material Science and NanoEngineering, Rice University, Houston, Texas 77005, USA*

In this Supplemental Material, we present calculations on the contribution of the topology of electronic bands to the phonon magnetic moment in  $\text{Pb}_{1-x}\text{Sn}_x\text{Te}$ , including different valleys and free carriers in real samples.

## PHONON MAGNETIC MOMENT FROM ELECTRONIC BAND TOPOLOGY

In this work, we experimentally studied chiral phonons in  $\text{Pb}_{1-x}\text{Sn}_x\text{Te}$  and found that these phonons exhibit a very strong phonon Zeeman effect indicating a giant phonon magnetic moment. Among the different mechanisms that can lead to large magnetic moment of phonons discussed in the main text, it was shown in Ref. [1] that the non-trivial band topology of electronic bands can impart a significant magnetic moment to chiral phonons. As discussed by the authors, this contribution is captured by the second Chern form. According to Eq. (3) in Ref. [1], the phonon magnetic moment is given by:

$$M_z = \frac{e}{2m_I} L_I \int d\mathbf{k} \Omega_{k_x k_y u_x u_y}, \quad (1)$$

where,  $m_I$  is the mass of the representative ion with averaged angular momentum  $L_I = (m_I/T) \int_0^T (\mathbf{u} \times \dot{\mathbf{u}} dt$  over the phonon period  $T$ ,  $k_\alpha$  and  $u_\alpha$  denote momentum and the displacement of phonon mode in  $\alpha$  direction with second Chern form

$$\Omega_{\alpha\beta\gamma\delta} = \Omega_{\alpha\beta}\Omega_{\gamma\delta} + \Omega_{\beta\gamma}\Omega_{\alpha\delta} - \Omega_{\alpha\gamma}\Omega_{\beta\delta}, \quad (2)$$

defined in terms of Berry curvature in  $\Omega_{\alpha\beta}$  in momentum ( $\mathbf{k}$ ) and phonon displacement ( $\mathbf{u}$ ) space.

## MODEL FOR LEAD TIN TELLURIDE

In order to calculate the band topology contribution to phononic magnetic moment, we consider the following effective four-band low-energy Hamiltonian around the L point [2]:

$$H_0 = (m + ck_3^2)\sigma_z + v(k_1s_y - k_2s_x)\sigma_x + v_3k_3\sigma_y, \quad (3)$$

where  $k_1, k_2, k_3$  form an orthogonal system with  $k_3$  pointing along  $\Gamma L$  line and  $k_1$  along the  $[110]$  direction. The point group at the L points is  $D_{3d}$  generated by inversion I, a  $C_3$  rotation about  $\Gamma L$  axis and mirror plane M. In the chosen coordinate system,  $k_1$  is perpendicular to the mirror plane, and  $k_3$  is along  $\Gamma L$  line. The corresponding

representations of the symmetry operators are as follows:

$$M = -is_x, k_1 \rightarrow -k_1 \quad (4)$$

$$R_3 = e^{i\pi/3}s_z, \vec{k} = R_3(2\pi/3)\vec{k} \quad (5)$$

$$I = \sigma_z, \vec{k} \rightarrow -\vec{k} \quad (6)$$

$$\Theta = is_yK, \vec{k} \rightarrow -\vec{k}. \quad (7)$$

If inversion, mirror, or  $C_3$  are broken by the phonon while preserving TRS, then at  $k_0$  order, we can incorporate the effect of phonons on electronic Hamiltonians by adding the following terms  $s_0\sigma_x, s_x\sigma_y, s_y\sigma_y, s_z\sigma_y$ . The action of these terms on different symmetries is shown in Table I.

|                    | $s_x\sigma_y$ | $s_y\sigma_y$ | $s_z\sigma_y$ | $s_0\sigma_x$ |
|--------------------|---------------|---------------|---------------|---------------|
| Inv ( $\sigma_z$ ) | ×             | ×             | ×             | ×             |
| $R_3$              | ×             | ×             | ✓             | ✓             |
| $M(=is_x)$         | ✓             | ×             | ×             | ✓             |
| $\Theta(=is_y)$    | ✓             | ✓             | ✓             | ✓             |

TABLE I. Action of different perturbation terms on symmetries of PbSnTe.

We considered many different combinations of these terms and found that one particular combination allows a non-zero phonon magnetic moment. In particular, the following form of electron-phonon interaction

$$H_{ph} = \zeta (u_x s_0 \sigma_x - u_y s_z \sigma_y), \quad (8)$$

where  $\zeta$  is electron-phonon coupling strength,  $u_x$  and  $u_y$  are phonon displacements associated with two linearly polarized orthogonal modes, results in a large phonon magnetic moment as shown in Fig. 1. Furthermore, the sign of magnetic moment depends on the sign of mass term as predicted in [1] and experimentally observed by us.

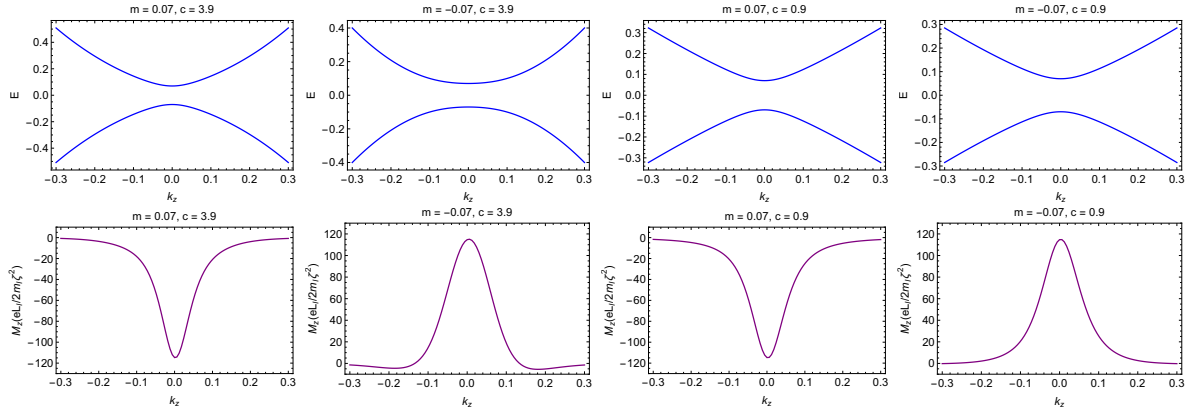

FIG. 1. Energy and phonon magnetic moment when only the lower bands are occupied for  $m = \pm 0.07$ ,  $v = 2.4$ ,  $v_3 = 0.95$ .

### Contribution from different valleys

Here, we are calculating the contribution of bulk band topology on phonon magnetic moment so we need to sum over all four  $L$  points (valleys). We can obtain the contribution from all different valleys by performing a  $C_4(z)$  which rotates the local  $k_1, k_2, k_3$  directions and also transforms the spin matrices ( $s_1 \rightarrow s_2, s_2 \rightarrow -s_1, s_3 \rightarrow s_3$ ). The phonon magnetic moment from all four valleys now point in local  $k_3$  direction. Although, as shown in table II the  $k.p$  hamiltonian around each value looks slightly different (it can be reduced to the same form if the  $x, y, z$  of spin matrices are also taken in the direction of local  $k_1, k_2, k_3$  direction) gives the same phonon magnetic moment along  $k_3$  for each valley. It shows that the phonon magnetic moment from different valleys should add up given that the form of  $H_{el-ph}$  term remains the same for all valleys.

| $L_i$                   | $\hat{\mathbf{k}}_1$  | $\hat{\mathbf{k}}_3$ | $k.p$                                                                 |
|-------------------------|-----------------------|----------------------|-----------------------------------------------------------------------|
| $L_1 (\pi, -\pi, \pi)$  | [110]                 | [1 $\bar{1}$ 1]      | $(m + ck_3^2)\sigma_z + v(k_1s_y - k_2s_x)\sigma_x + v_3k_3\sigma_y$  |
| $L_2 (\pi, \pi, \pi)$   | [ $\bar{1}$ 10]       | [111]                | $(m + ck_3^2)\sigma_z + v(-k_1s_x - k_2s_y)\sigma_x + v_3k_3\sigma_y$ |
| $L_3 (-\pi, \pi, \pi)$  | [ $\bar{1}\bar{1}$ 0] | [ $\bar{1}$ 11]      | $(m + ck_3^2)\sigma_z + v(-k_1s_y + k_2s_x)\sigma_x + v_3k_3\sigma_y$ |
| $L_4 (-\pi, -\pi, \pi)$ | [1 $\bar{1}$ 0]       | [ $\bar{1}$ 11]      | $(m + ck_3^2)\sigma_z + v(k_1s_x + k_2s_y)\sigma_x + v_3k_3\sigma_y$  |

TABLE II. Local  $k$  directions in terms of global directions and  $k.p$  for different valleys.

| Sample     | $m$ (meV) | $p$ ( $10^{18}cm^{-3}$ ) |
|------------|-----------|--------------------------|
| $x = 0$    | 100       | 0.26                     |
| $x = 0.24$ | 25        | 1.7                      |
| $x = 0.42$ | -20       | 8.1                      |
| $x = 0.56$ | -70       | 8.5                      |

TABLE III. Mass and carrier concentration for different samples.

### Consequences of a finite free carrier concentration on the phonon magnetic moment

It is well known that as the Sn content of  $Pb_{1-x}Sn_xTe$  samples is increased, the sign of the mass term at  $L$  point is inverted [3]. Additionally, it also increases the hole carrier concentration [4]. As shown in Fig. 2, this would result in a change in Fermi level which in turn affects the band occupancy around  $k_z = 0$  region. For a given sample, as the hole concentration keeps on increasing, the contribution to phonon magnetic moment from  $k_z = 0$  region is suppressed as shown in Fig. 3 for  $x = 0$  sample. It shows the predicted phonon magnetic moment can be different even for the same mass term value depending on the position of Fermi level. Now, when we consider samples with different Sn content, the position of Fermi level is influenced by the carrier concentration, mass ( $\Delta$ ) and Fermi velocities,  $v_F$  and  $v_3$  in  $k.p$  Hamiltonian of Eq. 3 which in turn decides the value of phonon magnetic moment as shown in Fig. 4 for  $x = 0$  and  $x = 0.24$  samples. This shows that the predicted  $1/\Delta^2$  dependence of the phonon magnetic moment [1] cannot be obtained in real  $Pb_{1-x}Sn_xTe$  samples, even for small  $x$  in the trivial side. In fact, if we consider the measured free carriers concentration in the samples with  $x=0$  and 0.24, together with the known bandgap dependence on  $x$ , it is possible for the ratio of phonon magnetic moment of  $x = 0$  and  $x = 0.24$  to attain a value closer to our experimental value of three for a reasonable value of Fermi velocity as shown in Fig. 5. Although, the values for variation of band gap with Sn doping are readily available, a similar analysis for Fermi velocities is somewhat lacking. Some recent works on Landau-level spectroscopy have measured Fermi velocity in  $Pb_{1-x}Sn_xTe$  samples but different works report different values. For example, ref. [5] reports a value of  $v_F = 7.3 \times 10^5 m/s$  (equivalent to 2.32 eV in our notation) for  $x = 0.46$  sample and ref. [6] uses a value of  $v_F = 2 \times 10^5 m/s$  (equivalent to 0.63 eV in our case) for  $x = 0.5$  sample. It prompted us to choose a range of Fermi velocities in order to calculate the phonon magnetic moment and we found that by using  $v_F \sim 1eV$  and  $v_3 \sim 0.5eV$ , the ratio of phonon magnetic moment for  $x = 0.24$  and  $x = 0$  comes close to the observed value of three.

Furthermore, the possibility to invert the sign of the mass term plays a crucial role in changing the topological properties of electronic bands. The band topology for SnTe is characterized by the mirror Chern number. If we consider a mirror plane  $\Gamma L_1 L_2$ , the total contribution to this mirror Chern number is not captured by the mirror Berry curvature in the vicinity of  $L_1$  and  $L_2$  points which indicates that there are other highsymmetry points (K,  $\Gamma$ ) on this plane which also contribute to mirror chern number. Now, the  $k.p$  model around  $L$  point cannot provide us this information and in fact, the statement that the SnTe has a band inversion happening at  $L$  points only indicates that the mirror Chern number for PbTe and SnTe differ by 2. It is important to note that this information is not sufficient to determine which one is topological. However, as discussed in Ref. [7], the presence of gapless surface states indicate that SnTe is topological. It can be understood as follows – the band inversion changes the mirror

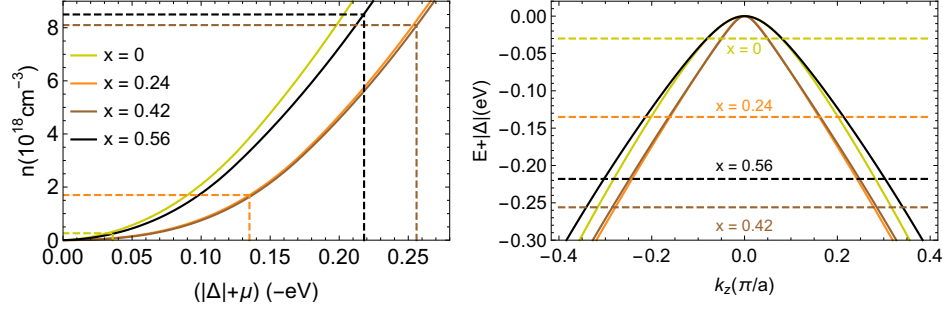

FIG. 2. Left: Carrier concentration as a function of chemical potential for  $\text{Pb}_{1-x}\text{Sn}_x\text{Te}$  samples with dashed lines showing the measured hole concentration of each sample. Right: Energy spectrum and the Fermi level for different samples with corresponding carrier concentration shown on left plot. We have used the band gap and hole concentration shown in Table III and Fermi velocities,  $v_F = 2.4\text{eV}$  and  $v_3 = 0.95\text{eV}$  ( $1\text{eV} \sim 3 \times 10^5\text{m/s}$  as we have considered lattice constant  $a \sim 6.5\text{\AA}$ ) is equivalent to and kept the same for all samples.

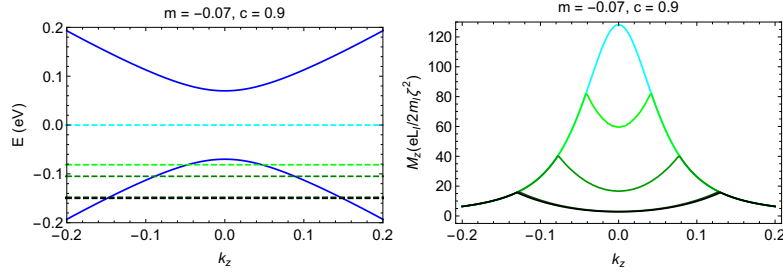

FIG. 3. Energy and phonon magnetic moment for different Fermi levels for  $m = -0.07$ ,  $v_F = 2.4\text{eV}$ ,  $v_3 = 0.95\text{eV}$ , and  $\zeta = 1$ .

Berry curvature at  $L$  points but the mirror Berry curvature in other regions on the mirror plane remains the same. It turns out that the mirror Berry curvature from other regions cancels out the mirror Berry curvature from  $L$  points for the case of PbTe. And, given that the mirror Berry curvature at  $L$  points differ by two for PbTe and SnTe case, we get a finite mirror Chern number for SnTe case. Now, in order to do a more concrete analysis, one should use a tight-binding model and obtain the full mirror Berry curvature profile for the given mirror plane. However, we can conclude that these regions won't contribute much to phonon magnetic moment as the band gap at these points is much larger than that at the  $L$  point [7]. As a result, it suffices to include only the  $L$  points for the purpose of calculating the electronic contribution to phonon magnetic moment.

Our model is based on bulk band topology and the predictions of this model in the regime,  $x > x_c$  fail to match the experimental observations. This could be due to the contribution from surface states which are absent on trivial side. However, our current model cannot be applied to gapless states and the (111) surface state are very robust to gap opening unlike (001) states which can be easily gapped out by rhombohedral distortion [2].

\* felixggh@if.usp.br

- [1] Y. Ren, C. Xiao, D. Saporov, and Q. Niu, Phonon Magnetic Moment from Electronic Topological Magnetization, *Phys. Rev. Lett.* **127**, 186403 (2021).
- [2] A. Lau and C. Ortix, Topological semimetals in the SnTe material class: Nodal lines and Weyl points, *Phys. Rev. Lett.* **122**, 186801 (2019).
- [3] J. O. Dimmock, I. Melngailis, and A. J. Strauss, Band Structure and Laser Action in  $\text{Pb}_x\text{Sn}_{1-x}\text{Te}$ , *Phys. Rev. Lett.* **16**, 1193 (1966).
- [4] E. Abramof, S. O. Ferreira, P. H. O. Rappl, H. Closs, and I. N. Bandeira, Electrical properties of  $\text{Pb}_{1-x}\text{Sn}_x\text{Te}$  layers with  $0 \leq x \leq 1$  grown by molecular beam epitaxy, *J. Appl. Phys.* **82**, 2405 (1997).
- [5] B. A. Assaf, T. Phuphachong, V. V. Volobuev, A. Inhofer, G. Bauer, G. Springholz, L. A. de Vaultier, and Y. Guldner, Massive and massless Dirac fermions in  $\text{Pb}_{1-x}\text{Sn}_x\text{Te}$  topological crystalline insulator probed by magneto-optical absorption, *Sci. Rep.* **6**, 20323 (2016).

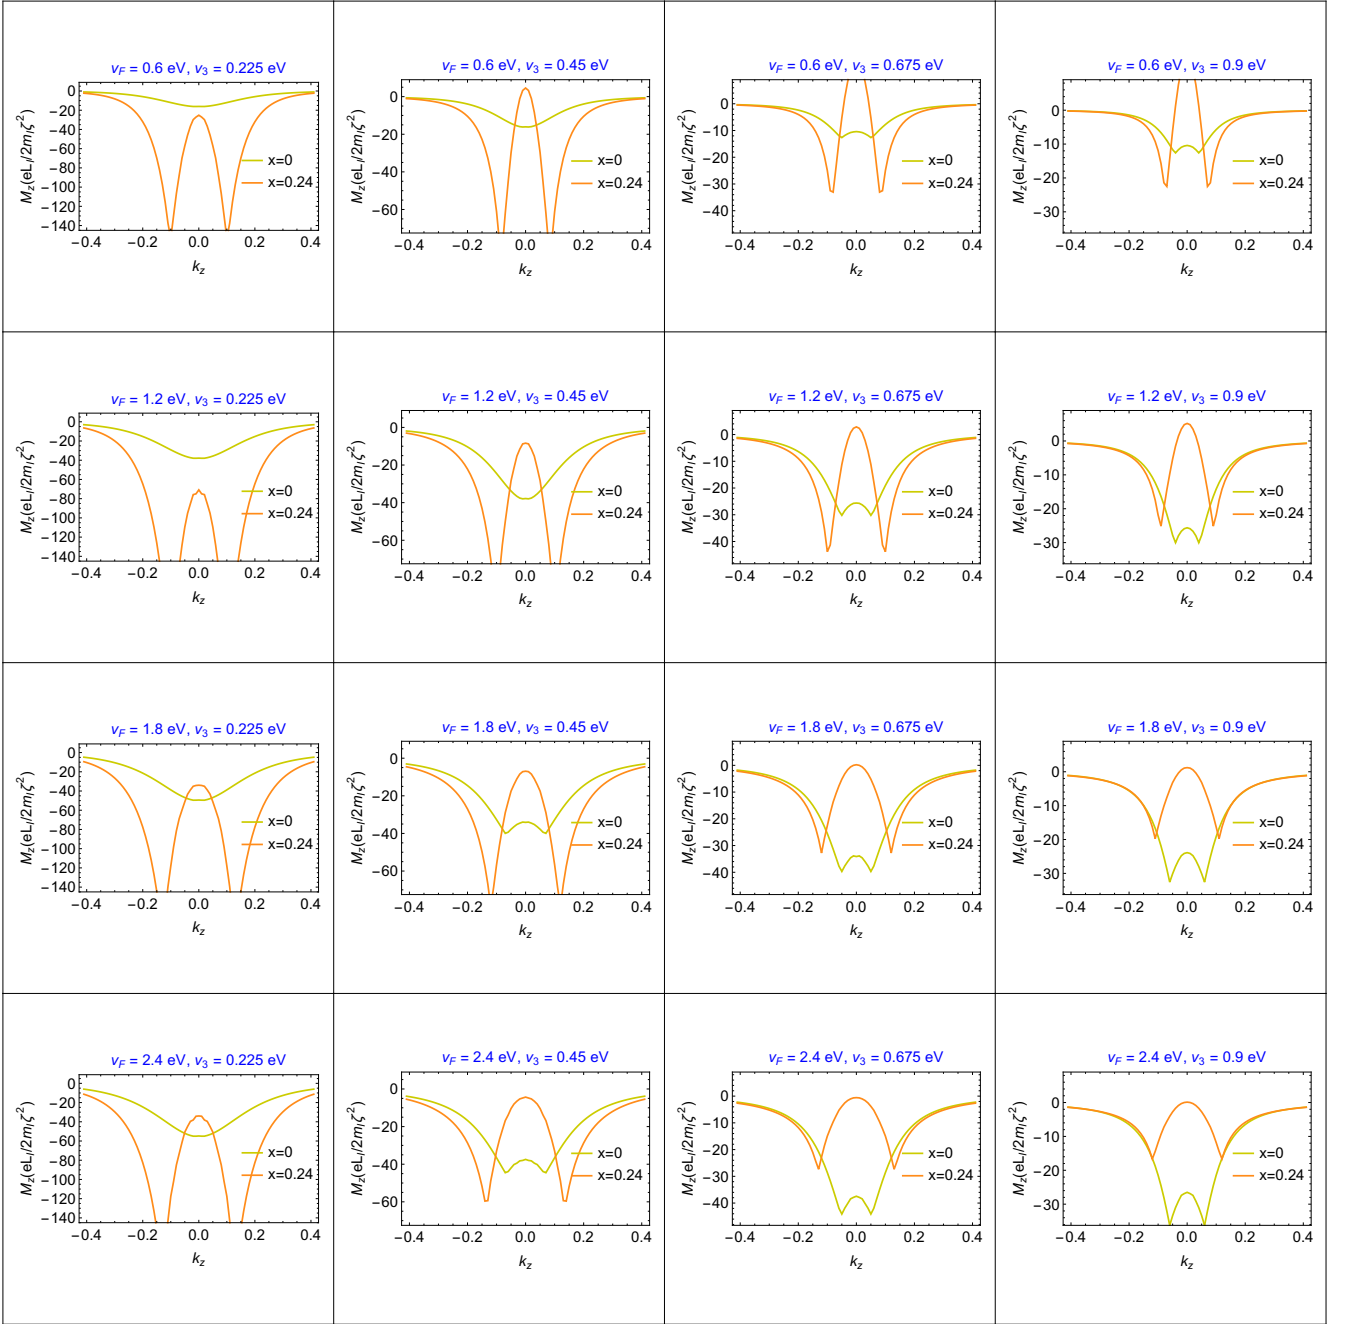

FIG. 4. The value of phonon magnetic moment of  $x = 0$  and  $x = 0.24$  sample for different values of Fermi velocities. This calculation was assuming a bandgap of 200 and 50 meV and the measured hole concentration of  $2.6 \times 10^{17} \text{ cm}^{-3}$  and  $1.7 \times 10^{18} \text{ cm}^{-3}$  for  $x = 0$  and  $x = 0.24$  samples, respectively. The Fermi velocities are given in units of eV

- [6] B. Cheng, P. Taylor, P. Folkes, C. Rong, and N. P. Armitage, Magnetoterahertz Response and Faraday Rotation from Massive Dirac Fermions in the Topological Crystalline Insulator  $\text{Pb}_{0.5}\text{Sn}_{0.5}\text{Te}$ , *Phys. Rev. Lett.* **122**, 097401 (2019).
- [7] T. H. Hsieh, H. Lin, J. Liu, W. Duan, A. Bansil, and L. Fu, Topological crystalline insulators in the SnTe material class, *Nat. Comm.* **3**, 982 (2012).

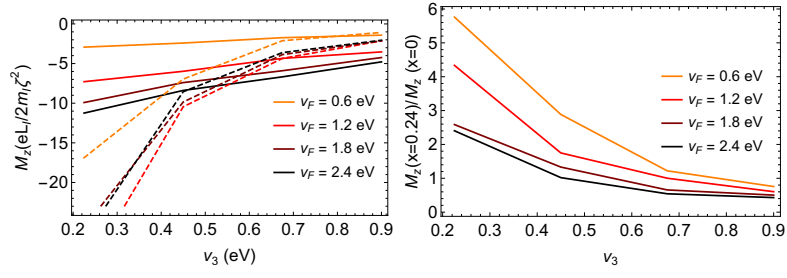

FIG. 5. Left: The value of phonon magnetic moment of  $x = 0$  (solid lines) and  $x = 0.24$  (dashed lines) integrated over  $k_z$  as a function of Fermi velocity. Right: The ratio of phonon magnetic moment for those two samples.
